# Supplementary material for: Excitons and Optical Response in Excitonic Insulator Candidate TiSe$_2$
Source: arXiv:2510.00556 ancillary file (2026-02-24)
Supplement: Supplementary file 1 [file SM.pdf]

# Supplemental Material:

## Excitons and Optical Response in Excitonic Insulator Candidate $\text{TiSe}_2$

Dino Novko<sup>1,2,\*</sup>

<sup>1</sup>*Centre for Advanced Laser Techniques, Institute of Physics, 10000 Zagreb, Croatia*

<sup>2</sup>*Donostia International Physics Center (DIPC), 20018 Donostia-San Sebastián, Spain*

### S1. COMPUTATIONAL DETAILS

The density functional theory (DFT) calculations of the ground state, needed for the linear response and Bethe-Salpeter equation (BSE) calculations, were performed with the GPAW package [S1]. The plane-wave basis set with the energy cutoff of 45 Ry and Perdew–Burke–Ernzerhof (PBE) exchange–correlation functional were used. In order to obtain a more accurate description of the electronic structure we use the hybrid functional HSE0 [S2] as well as the GW approach [S3]. The atomic positions were relaxed until the forces were below  $10^{-6}$  Ry/ $a_0$ . The unit cell parameter of  $\text{TiSe}_2$  was set to the PBE-derived value of 3.5473 Å, which is close to the experimental value of 3.54 Å. The distance between Ti and Se atomic planes are relaxed to the value of 1.549 Å. In order to get the PLDs and CDW structures, we perform the relaxation of the atomic position in  $2 \times 2$  cell for each temperature (entering the Fermi-Dirac broadening function). With that procedure we get that  $T_{\text{CDW}}^{\text{PBE}} = 1100$  K  $T_{\text{CDW}}^{\text{HSE}} = 2000$  K. For each of these structures, including the  $1 \times 1$  normal unit cell, we perform the BSE and optical absorption calculations.

The momentum grid for ground-state density calculations of normal  $1 \times 1$  phase of  $\text{TiSe}_2$  was  $\mathbf{k} = 48 \times 48 \times 1$ . In the calculations of the screened Coulomb propagator (linear response calculations) we use 40 electronic bands [S4]. The BSE calculations for the normal phase are done on the same momentum grid and 4 bands are involved in the diagonalization (2 conduction Se- $p$  states and 2 valence Ti- $d$  states). The G0W0 calculations for  $1 \times 1$  normal phase were done on the same momentum grid, using also 40 bands for linear response, and with a planewave energy cut off of 50 eV. The G0W0 correction was done on the same 4 bands that are afterwards used in the BSE calculations.

The momentum grid for ground-state density calculations of the CDW  $2 \times 2$  phase of  $\text{TiSe}_2$  was  $\mathbf{k} = 24 \times 24 \times 1$ . Here the calculations of the screened Coulomb propagator were done with 110 electronic bands. The corresponding BSE calculations for the CDW structures were done on the same momentum grid and we included 7 bands in the diagonalization of the BSE Hamiltonian (3 conduction Se- $p$  states and 4 valence Ti- $d$  states). The broadening parameter used in the optical absorption calculations was set to 80 meV. The G0W0 calculations for  $2 \times 2$  CDW structures were done on the same  $24 \times 24 \times 1$  momentum grid, using also 110 bands for linear response, and with a planewave energy cut off of 20 eV.

In the HSE+BSE calculations we use actually the PBE+BSE approach where we correct the band gap with a scissor method to match the HSE electronic band gap.

---

\* [dino.novko@gmail.com](mailto:dino.novko@gmail.com)

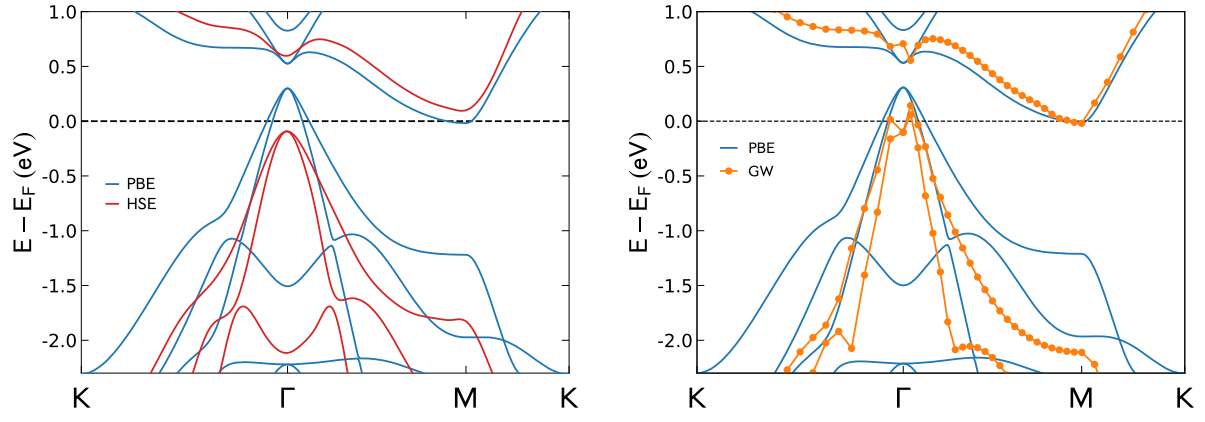

FIG. S1. Electronic band structure of normal high-temperature phase of  $\text{TiSe}_2$  as obtained with PBE and HSE functionals, as well as with GW quasi-particle corrections.

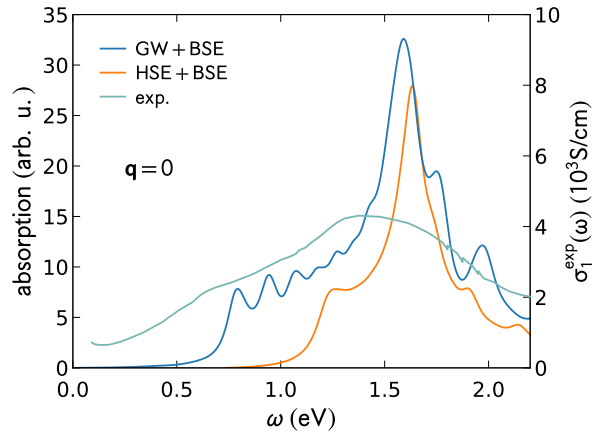

FIG. S2. Optical absorption spectra for the normal high-temperature phase of  $\text{TiSe}_2$  as obtained with GW+BSE and HSE+BSE methods. In the GW+BSE approach the BSE are done on top of the GW band structure. For HSE+BSE approach the scissor method is applied to correct for the right band gap between the Se- $p$  and Ti- $d$  states at the M point of the Brillouin zone. The experimental optical absorption data are from Ref. [S5] done for  $T > T_{\text{CDW}}$ .

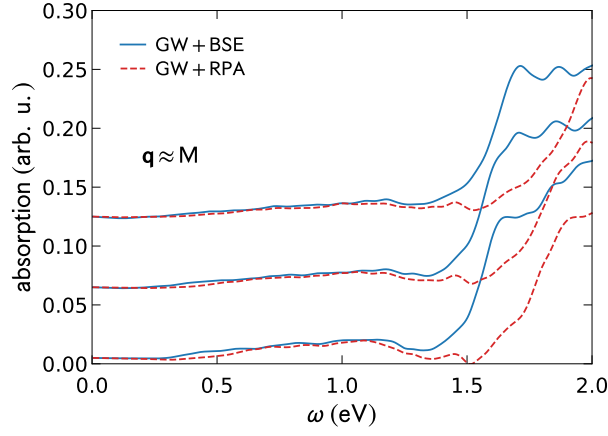

FIG. S3. Electron excitation spectra for the normal high-temperature phase of  $\text{TiSe}_2$  for momenta close to the M point. These results are done with GW+BSE and PBE+BSE approaches.

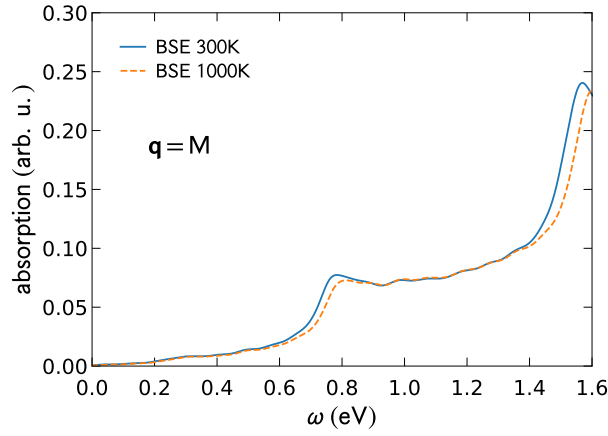

FIG. S4. Electron excitation spectrum for the normal high-temperature phase of  $\text{TiSe}_2$  for  $\mathbf{q} = \mathbf{M}$  done with PBE+BSE and for  $T=300$  K and  $T=1000$  K. Here we use a denser  $\mathbf{k}$ -grid of  $90 \times 90 \times 1$  to get a better results for the 300 K temperature, however, in order to reduce the numerical cost, we use only 3 states around the Fermi level (1 Ti- $d$  and 2 Se- $p$  states) for the diagonalization of the BSE Hamiltonian.

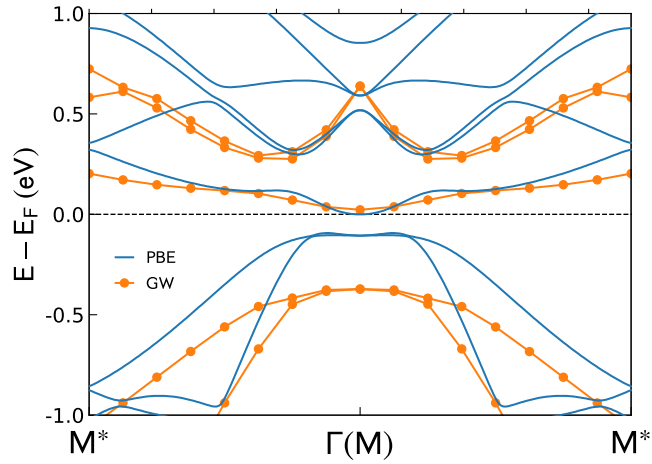

FIG. S5. Electronic band structure of the  $2 \times 2$  CDW phase of  $\text{TiSe}_2$  as obtained with PBE functionals and with GW quasi-particle correction.

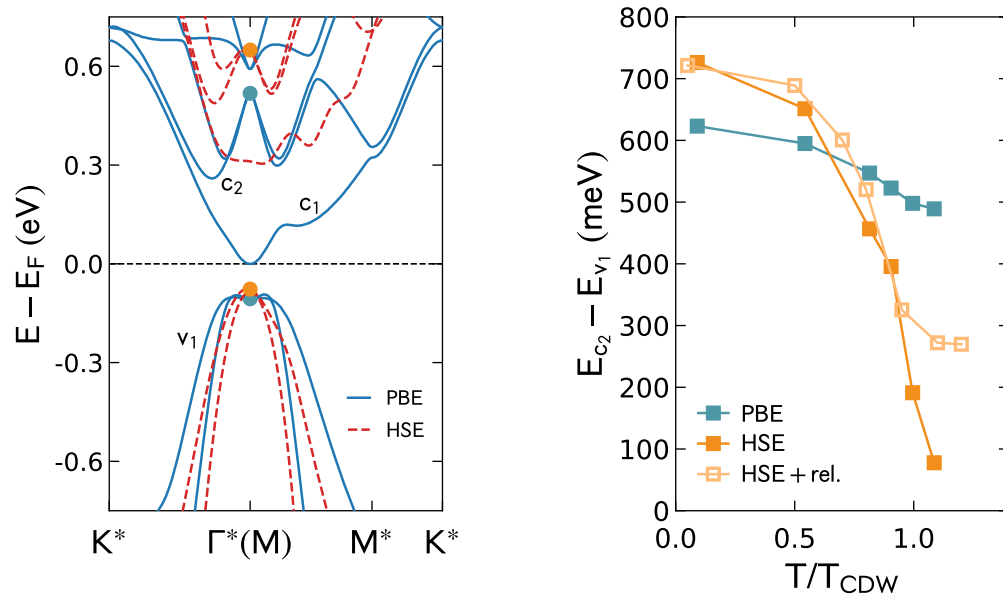

FIG. S6. (Left) Electronic band structure of  $\text{TiSe}_2$  in the CDW phase at 100 K as obtained with PBE and HSE functionals. (Right) The CDW gap opening as a function of temperature. The evaluated CDW gap for HSE and PBE electronic structures is shown with orange and blue dots in the left panel. Full orange squares are for the HSE calculations of the band structure, but the unit cell and periodic lattice distortions are relaxed for each temperature with PBE functional. Open orange squares are for the results where both electronic structure and PLDs are done with HSE functional. In the first case  $T_{\text{CDW}}^{\text{PBE}} = 1100$  K, while in the second case we get  $T_{\text{CDW}}^{\text{HSE}} = 2000$  K.

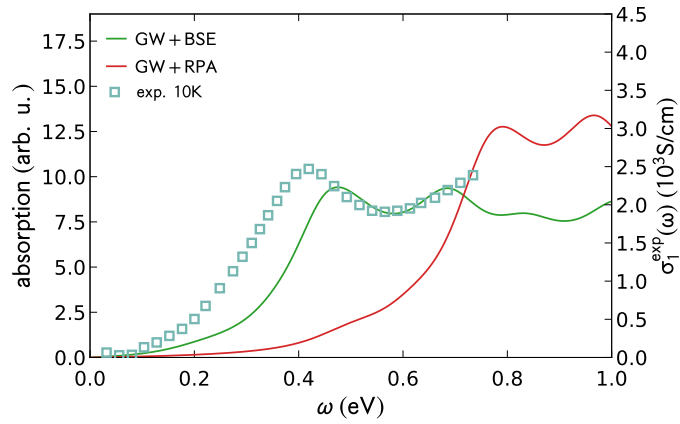

FIG. S7. Optical absorption spectra for the CDW phase at low temperatures as obtained with GW+BSE and GW+RPA methods. The experimental results are from Ref. S5.

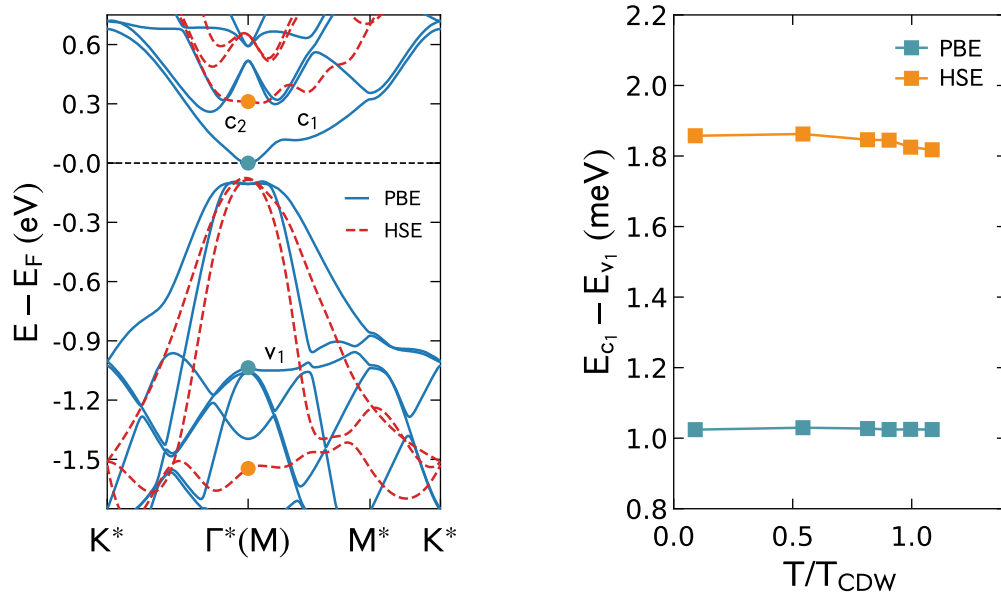

FIG. S8. (Left) Electronic band structure of  $\text{TiSe}_2$  in the CDW phase at 100 K as obtained with PBE and HSE functionals. (Right) The high-energy gap between  $c_1$  (Ti- $d$ ) state at  $\Gamma^*(\Gamma)$  and  $v_1$  (Se- $p$ ) at  $\Gamma^*(M)$  obtained with PBE and HSE functionals and as a function of temperature. The evaluated high-energy gap for HSE and PBE electronic structures is shown with orange and blue dots in the left panel.

#### SUPPLEMENTAL REFERENCES

- [S1] J. Enkovaara, C. Rostgaard, J. J. Mortensen, J. Chen, M. Dułak, L. Ferrighi, J. Gavnholt, C. Glinsvad, V. Haikola, H. A. Hansen, H. H. Kristoffersen, M. Kuisma, A. H. Larsen, L. Lehtovaara, M. Ljungberg, O. Lopez-Acevedo, P. G. Moses, J. Ojanen, T. Olsen, V. Petzold, N. A. Romero, J. Stausholm-Møller, M. Strange, G. A. Tritsarlis, M. Vanin, M. Walter, B. Hammer, H. Häkkinen, G. K. H. Madsen, R. M. Nieminen, J. K. Nørskov, M. Puska, T. T. Rantala, J. Schiøtz, K. S. Thygesen, and K. W. Jacobsen, *Journal of Physics: Condensed Matter* **22**, 253202 (2010).
- [S2] J. Heyd, G. E. Scuseria, and M. Ernzerhof, *The Journal of Chemical Physics* **118**, 8207 (2003).
- [S3] F. Hüser, T. Olsen, and K. S. Thygesen, *Phys. Rev. B* **87**, 235132 (2013).
- [S4] J. Yan, J. J. Mortensen, K. W. Jacobsen, and K. S. Thygesen, *Phys. Rev. B* **83**, 245122 (2011).
- [S5] G. Li, W. Z. Hu, D. Qian, D. Hsieh, M. Z. Hasan, E. Morosan, R. J. Cava, and N. L. Wang, *Phys. Rev. Lett.* **99**, 027404 (2007).
